# Supplementary material for: Learning-to-Optimize with PAC-Bayesian Guarantees: Theoretical Considerations and Practical Implementation
Source: arXiv:2404.03290 source file (2025-02-25)
Supplement: Supplementary file 1 [file Supplementary_Material.tex]

\subsection{On the Finiteness Assumption of $\Lambda$} 

We denote the open ball of radius $r$ around a point $x$ by $\mathcal{B}(x; r)$ and the corresponding closed ball by $\mathcal{B}[x; r]$. For a set $S$, the notation $\vert S \vert$ denotes the cardinality of $S$.

\begin{Def}[Totally Bounded Space]
    A metric space $(\space{X}, d)$ is called \emph{totally bounded}, if for every $\epsilon > 0$ there exists $n \in \mathbb{N}$, $x_1,...,x_n \in \space{X}$, such that
    $$
        \space{X} \subseteq \bigcup_{i=1}^n \mathcal{B}(x_i;\epsilon) \,.
    $$
\end{Def}

The typical example of a totally bounded space is a compact space. The important property of this space, which is used in the following, is that they have a finite covering number. In the end, this allows again to apply the union bound argument.

\begin{Def}[$\delta$-Covering Number]
    Let $(\space{X}, d)$ be a totally bounded metric space and let $\delta > 0$. A \emph{proper $\delta$-covering} of $\space{X}$ is a finite set $X_\delta \subset \space{X}$, such that
    $$
        \space{X} \subseteq \bigcup_{x \in X_\delta} \mathcal{B}[x;\delta] \,.
    $$
    The minimal cardinality of any $\delta$-covering is denoted $\coveringNumber{\delta}{\space{X}}$ and is called the \emph{$\delta$-covering number} of $\space{X}$:
    $$
        \coveringNumber{\delta}{\space{X}} := \min \{\vert X_\delta \vert \ : \ \text{$X_\delta$ is a proper $\delta$-covering of $\space{X}$}\} \,.
    $$
\end{Def}

Taken together, and using the proof of Theorem \ref{Thm_PACBayes_exponential_familiy} as entry point, one gets the following Lemma. This is a direct generalization of the result in Theorem \ref{Thm_PACBayes_exponential_familiy}, as in the case where $\Lambda$ is finite, $\Lambda$ can be covered by itself, such that it holds $\coveringNumber{\delta}{\Lambda} = \vert \Lambda \vert$ and $C = 0$.

\begin{Lem}\label{proof_LambdaFiniteNotNecessary}
    Let $(\Lambda, d)$ be a totally bounded metric space and let $\delta > 0$. Assume that there is a constant $C(\delta)$, such that for all $\Tilde{\lambda} \in \Lambda$ and $d \in \space{D}_N$ it holds: 
    $$
    \sup_{\lambda \in \closedBall{\Tilde{\lambda}}{\delta}} \kappa_d(\lambda) - \kappa_d(\Tilde{\lambda}) \le C(\delta) \,.
    $$
    Finally, assume that $\mathbb{P} \{ \kappa(\lambda, \rvec{D}_N) > s  \} \le \exp(-s)$ for all $s \in \mathbb{R}$, $\lambda \in \Lambda$. Then it holds that:
    $$
        \mathbb{P} \Bigl\{ \sup_{\lambda \in \Lambda} \kappa(\lambda, \rvec{D}_N) \le \log \Bigl( \frac{\coveringNumber{\delta}{\Lambda}}{\epsilon} \Bigr) + C(\delta) \Bigr\} \ge 1-\epsilon \,.
    $$
\end{Lem}
\begin{proof}
    Since $(\Lambda, d)$ is a totally bounded metric space, its covering number $\coveringNumber{\delta}{\Lambda}$ is well-defined and finite. For notational simplicity, set $N := \coveringNumber{\delta}{\Lambda}$. Hence, there are $\lambda_1, ..., \lambda_N \in \Lambda$, such that:
    $$
        \Lambda \subseteq \bigcup_{i=1}^N \closedBall{\lambda_i}{\delta} \,.
    $$
    Therefore, one directly gets for every $d \in \space{D}_N$:
    $$
        \sup_{\lambda \in \Lambda} \kappa_d(\lambda) \le \max_{i=1,...,N} \ \sup_{\lambda \in \closedBall{\lambda_i}{\delta}} \kappa_d(\lambda) \,.
    $$
    Further, by assumption it holds:
    $$
        \sup_{\lambda \in \closedBall{\lambda_i}{\delta}} \kappa_d(\lambda) 
        = \kappa_d(\lambda_i) + \sup_{\lambda \in \closedBall{\lambda_i}{\delta}} \Bigr(\kappa_d(\lambda) - \kappa_d(\lambda_i) \Bigl) 
        \le \kappa_d(\lambda_i) + C(\delta) \,.
    $$
    Hence, in total one gets for $s \in \mathbb{R}$:
    \begin{align*}
        \prob \left\{ \sup_{\lambda \in \Lambda} \kappa(\lambda, \rvec{D}_N) > s \right\} 
        &\le \prob \left\{ \max_{i=1,...,N} \kappa(\lambda_i, \rvec{D}_N) + C(\delta) > s \right\}  \\
        &= \prob \bigcup_{i=1}^N \{\kappa(\lambda_i, \rvec{D}_N) + C(\delta) > s\} \\
        &\le \sum_{i=1}^N \prob \left\{ \kappa(\lambda_i, \rvec{D}_N) + C(\delta) > s \right\} \\
        &\le \sum_{i=1}^N \exp(C(\delta)-s) \\
        &= N \exp(C(\delta)-s) \,.
    \end{align*}
    Since $\epsilon = N \exp(C-s) \ \iff s = \log\left( \frac{N}{\epsilon} \right) + C(\delta)$, one gets:
    $$
    \mathbb{P} \left\{ \sup_{\lambda \in \Lambda} \kappa(\lambda, \rvec{D}_N) > \log\left( \frac{N}{\epsilon} \right) + C(\delta) \right\} \le \epsilon\,.
    $$
    Taking the complementary event yields the result:
    $$
    \mathbb{P} \left\{ \sup_{\lambda \in \Lambda} \kappa(\lambda, \rvec{D}_N) \le \log\left( \frac{N}{\epsilon} \right) + C(\delta) \right\} \ge 1-\epsilon\,.
    $$
\end{proof}

\begin{Rem}
    One typical example, for which the assumption 
    $$
    \sup_{\lambda \in \closedBall{\Tilde{\lambda}}{\delta}} \kappa_d(\lambda) - \kappa_d(\Tilde{\lambda}) \le C(\delta)
    $$ is verified easily, is the case when $\kappa$ is continuous. In this case, by restricting $\Lambda$ to a compact set, one can take $\kappa$ to be Lipschitz-continuous with some constant $L \ge 0$, which, by definition guarantees the corresponding growth condition with $C(\delta) = L \delta$.
\end{Rem}
